# Supplementary material for: SL$^{2}$A-INR: Single-Layer Learnable Activation for Implicit Neural Representation
Source: arXiv:2409.10836 source file (2025-09-30)
Supplement: Supplementary file 1 [file main_supp.tex]

% ICCV 2025 Paper Template

\documentclass[10pt,twocolumn,letterpaper]{article}

%%%%%%%%% PAPER TYPE  - PLEASE UPDATE FOR FINAL VERSION
\usepackage{iccv}   
\pagenumbering{gobble}% To produce the CAMERA-READY version
% \usepackage[pagenumbers]{iccv}      % To produce the REVIEW version
% \usepackage[pagenumbers]{iccv} % To force page numbers, e.g. for an arXiv version

% Import additional packages in the preamble file, before hyperref
\input{preamble}

% It is strongly recommended to use hyperref, especially for the review version.
% hyperref with option pagebackref eases the reviewers' job.
% Please disable hyperref *only* if you encounter grave issues, 
% e.g. with the file validation for the camera-ready version.
%
% If you comment hyperref and then uncomment it, you should delete *.aux before re-running LaTeX.
% (Or just hit 'q' on the first LaTeX run, let it finish, and you should be clear).
\definecolor{iccvblue}{rgb}{0.21,0.49,0.74}
\usepackage[pagebackref,breaklinks,colorlinks,allcolors=iccvblue]{hyperref}
\usepackage{booktabs} % For professional-looking tables (\toprule, \midrule, \bottomrule)
\usepackage{multirow} % For multi-row elements in tables
\usepackage{graphicx} % For rotating text
\usepackage{colortbl} % For cell coloring
\usepackage{xcolor} % For defining colors

%%%%%%%%% PAPER ID  - PLEASE UPDATE
 % *** Enter the Paper ID here

% %%%%%%%%% TITLE - PLEASE UPDATE
% \title{SL$^{2}$A-INR: Single-Layer Learnable Activation for Implicit Neural Representation}
% %%%%%%%%% AUTHORS - PLEASE UPDATE
% \author{First Author\\
% Institution1\\
% Institution1 address\\
% {\tt\small firstauthor@i1.org}
% % For a paper whose authors are all at the same institution,
% % omit the following lines up until the closing ``}''.
% % Additional authors and addresses can be added with ``\and'',
% % just like the second author.
% % To save space, use either the email address or home page, not both
% \and
% Second Author\\
% Institution2\\
% First line of institution2 address\\
% {\tt\small secondauthor@i2.org}
% }
% \title{SL$^{2}$A-INR: Single-Layer Learnable Activation for Implicit Neural Representation}

% \author{
% Reza Rezaeian\thanks{Equal contribution.}\\
% University of Tehran
% \and
% Moein Heidari\footnotemark[1]\\
% University of British Columbia
% \and
% Reza Azad\\
% RWTH Aachen University
% \and
% Dorit Merhof\\
% University of Regensburg
% \and
% Hamid Soltanian-Zadeh\thanks{Corresponding author. Email: hszadeh@ut.ac.ir.}\\
% University of Tehran
% \and
% Ilker Hacihaliloglu\thanks{Corresponding author. Email: ilker.hacihaliloglu@ubc.ca.}\\
% University of British Columbia
% }

\begin{document}
% \maketitle
\input{SL2A/sec/7_supplementary}

\newpage
{
    \small
    \bibliographystyle{ieeenat_fullname}
    \bibliography{main}
}

\end{document}
